# Supplementary material for: Quantum Circuit Transformation: A Monte Carlo Tree Search Framework
Source: arXiv:2008.09331 source file (2022-01-25)
Supplement: Supplementary file 1 [file appendix.tex]

\onecolumn

\section{Qiskit Quantum Circuits Set Benchmarks}

\footnotesize
% Please add the following required packages to your document preamble:
% \usepackage{longtable}
% Note: It may be necessary to compile the document several times to get a multi-page table to line up properly

\begin{longtable}[c]{cccccccc}
\caption{Detailed results of MCTS-Size and MCTS-Size+r on IBM Q20 with naive initial mappings (Circuits are extracted from Qiskit library and each SWAP is decomposed into 3 CNOTs).}\\
%\scalebox{0.9}{
\hline
\begin{tabular}[c]{@{}c@{}}Circuit\\      Name\end{tabular} & \begin{tabular}[c]{@{}c@{}}\#gate\\      input\end{tabular} & \begin{tabular}[c]{@{}c@{}}\#cnot\\      input\end{tabular} & \begin{tabular}[c]{@{}c@{}}depth\\      input\end{tabular} & \begin{tabular}[c]{@{}c@{}}\#gate\\      mcts-s\end{tabular} & \begin{tabular}[c]{@{}c@{}}depth\\      mcts-s\end{tabular} & \begin{tabular}[c]{@{}c@{}}\#gate\\      mcts-s+r\end{tabular} & \begin{tabular}[c]{@{}c@{}}depth\\      mcts-s+r\end{tabular} \\
%\endfirsthead
%
\hline
\endhead
AND\_10 & 3067 & 1532 & 2556 & 3199 & 2584 & 3241 & 2674 \\
AND\_11 & 6139 & 3068 & 5116 & 6397 & 5239 & 6331 & 5233 \\
AND\_12 & 12283 & 6140 & 10236 & 13000 & 10292 & 12763 & 10544 \\
AND\_13 & 24571 & 12284 & 20476 & 25765 & 20506 & 25411 & 21004 \\
AND\_14 & 49147 & 24572 & 40956 & 50998 & 40983 & 50740 & 41985 \\
AND\_5 & 105 & 36 & 81 & 123 & 84 & 123 & 94 \\
AND\_6 & 187 & 92 & 156 & 217 & 174 & 214 & 170 \\
AND\_7 & 379 & 188 & 316 & 433 & 332 & 421 & 340 \\
AND\_8 & 763 & 380 & 636 & 847 & 678 & 832 & 676 \\
AND\_9 & 1531 & 764 & 1276 & 1675 & 1302 & 1633 & 1324 \\
excitation\_preserving\_10 & 1930 & 540 & 374 & 2140 & 898 & 2146 & 978 \\
excitation\_preserving\_11 & 2354 & 660 & 414 & 2633 & 1303 & 2639 & 1250 \\
excitation\_preserving\_12 & 2820 & 792 & 454 & 3114 & 1477 & 3117 & 1443 \\
excitation\_preserving\_13 & 3328 & 936 & 494 & 3691 & 1807 & 3697 & 1762 \\
excitation\_preserving\_14 & 3878 & 1092 & 534 & 4286 & 1973 & 4271 & 1919 \\
excitation\_preserving\_15 & 4470 & 1260 & 574 & 4944 & 2240 & 5010 & 2359 \\
excitation\_preserving\_5 & 440 & 120 & 174 & 485 & 285 & 476 & 265 \\
excitation\_preserving\_6 & 654 & 180 & 214 & 717 & 423 & 717 & 423 \\
excitation\_preserving\_7 & 910 & 252 & 254 & 1003 & 480 & 1003 & 480 \\
excitation\_preserving\_8 & 1208 & 336 & 294 & 1340 & 694 & 1340 & 694 \\
excitation\_preserving\_9 & 1548 & 432 & 334 & 1728 & 769 & 1728 & 756 \\
grover\_operator\_10 & 3110 & 1532 & 2562 & 3242 & 2590 & 3281 & 2680 \\
grover\_operator\_11 & 6186 & 3068 & 5122 & 6444 & 5245 & 6378 & 5239 \\
grover\_operator\_12 & 12334 & 6140 & 10242 & 13051 & 10299 & 12754 & 10486 \\
grover\_operator\_13 & 24626 & 12284 & 20482 & 25820 & 20512 & 25778 & 21168 \\
grover\_operator\_14 & 49206 & 24572 & 40962 & 51057 & 40989 & 50799 & 41991 \\
grover\_operator\_5 & 128 & 36 & 87 & 146 & 90 & 146 & 102 \\
grover\_operator\_6 & 214 & 92 & 162 & 244 & 179 & 241 & 175 \\
grover\_operator\_7 & 410 & 188 & 322 & 464 & 339 & 452 & 346 \\
grover\_operator\_8 & 798 & 380 & 642 & 888 & 666 & 867 & 682 \\
grover\_operator\_9 & 1570 & 764 & 1282 & 1714 & 1309 & 1672 & 1330 \\
hidden\_linear\_10 & 68 & 16 & 21 & 98 & 45 & 101 & 45 \\
hidden\_linear\_11 & 76 & 18 & 23 & 118 & 61 & 115 & 43 \\
hidden\_linear\_12 & 84 & 20 & 25 & 123 & 57 & 126 & 51 \\
hidden\_linear\_13 & 92 & 22 & 27 & 137 & 66 & 134 & 61 \\
hidden\_linear\_14 & 100 & 24 & 29 & 148 & 64 & 145 & 57 \\
hidden\_linear\_15 & 108 & 26 & 31 & 162 & 66 & 159 & 64 \\
hidden\_linear\_5 & 28 & 6 & 11 & 43 & 26 & 40 & 28 \\
hidden\_linear\_6 & 36 & 8 & 13 & 57 & 28 & 57 & 28 \\
hidden\_linear\_7 & 44 & 10 & 15 & 62 & 36 & 62 & 36 \\
hidden\_linear\_8 & 52 & 12 & 17 & 73 & 39 & 73 & 33 \\
hidden\_linear\_9 & 60 & 14 & 19 & 87 & 40 & 90 & 46 \\
inner\_product\_10 & 15 & 5 & 3 & 15 & 3 & 15 & 3 \\
inner\_product\_12 & 18 & 6 & 3 & 33 & 17 & 33 & 17 \\
inner\_product\_14 & 21 & 7 & 3 & 39 & 11 & 39 & 11 \\
inner\_product\_6 & 9 & 3 & 3 & 21 & 11 & 21 & 11 \\
inner\_product\_8 & 12 & 4 & 3 & 24 & 14 & 24 & 14 \\
integer\_comparator\_10 & 110 & 42 & 73 & 134 & 82 & 134 & 82 \\
integer\_comparator\_12 & 140 & 54 & 93 & 182 & 114 & 182 & 123 \\
integer\_comparator\_14 & 170 & 66 & 113 & 224 & 136 & 227 & 160 \\
integer\_comparator\_6 & 50 & 18 & 33 & 65 & 43 & 65 & 43 \\
integer\_comparator\_8 & 80 & 30 & 53 & 95 & 62 & 95 & 62 \\
IQP\_10 & 225 & 78 & 72 & 294 & 155 & 294 & 179 \\
IQP\_11 & 276 & 98 & 79 & 363 & 196 & 363 & 186 \\
IQP\_12 & 319 & 114 & 84 & 415 & 247 & 418 & 197 \\
IQP\_13 & 364 & 130 & 92 & 469 & 224 & 481 & 258 \\
IQP\_14 & 430 & 156 & 104 & 547 & 286 & 562 & 329 \\
IQP\_15 & 483 & 176 & 104 & 642 & 285 & 648 & 327 \\
IQP\_5 & 60 & 18 & 32 & 78 & 48 & 78 & 48 \\
IQP\_6 & 88 & 28 & 40 & 118 & 77 & 118 & 77 \\
IQP\_7 & 116 & 38 & 48 & 152 & 88 & 149 & 87 \\
IQP\_8 & 163 & 56 & 56 & 202 & 112 & 202 & 112 \\
IQP\_9 & 191 & 66 & 60 & 242 & 143 & 245 & 120 \\
OR\_10 & 3086 & 1532 & 2557 & 3218 & 2585 & 3263 & 2672 \\
OR\_11 & 6160 & 3068 & 5117 & 6418 & 5240 & 6352 & 5234 \\
OR\_12 & 12306 & 6140 & 10237 & 13023 & 10293 & 12726 & 10481 \\
OR\_13 & 24596 & 12284 & 20477 & 25790 & 20507 & 25433 & 21008 \\
OR\_14 & 49174 & 24572 & 40957 & 51025 & 40984 & 50767 & 41986 \\
OR\_5 & 114 & 36 & 82 & 132 & 85 & 132 & 85 \\
OR\_6 & 198 & 92 & 157 & 228 & 175 & 225 & 171 \\
OR\_7 & 392 & 188 & 317 & 446 & 333 & 434 & 341 \\
OR\_8 & 778 & 380 & 637 & 862 & 679 & 847 & 677 \\
OR\_9 & 1548 & 764 & 1277 & 1692 & 1303 & 1650 & 1325 \\
phase\_estimation\_10 & 3981 & 1586 & 2604 & 4071 & 2673 & 4071 & 2673 \\
phase\_estimation\_11 & 7863 & 3138 & 5172 & 7956 & 5259 & 7956 & 5257 \\
phase\_estimation\_12 & 15590 & 6228 & 10300 & 15701 & 10386 & 15704 & 10397 \\
phase\_estimation\_13 & 31002 & 12392 & 20548 & 31131 & 20702 & 31125 & 20730 \\
phase\_estimation\_5 & 126 & 48 & 84 & 153 & 96 & 153 & 99 \\
phase\_estimation\_6 & 263 & 102 & 172 & 290 & 190 & 290 & 190 \\
phase\_estimation\_7 & 525 & 206 & 340 & 570 & 372 & 567 & 369 \\
phase\_estimation\_8 & 1032 & 408 & 668 & 1077 & 691 & 1074 & 695 \\
phase\_estimation\_9 & 2024 & 804 & 1316 & 2087 & 1361 & 2090 & 1373 \\
phase\_oracle\_10 & 896 & 380 & 636 & 986 & 660 & 944 & 668 \\
phase\_oracle\_11 & 3586 & 1532 & 2556 & 3745 & 2652 & 3700 & 2624 \\
phase\_oracle\_12 & 3586 & 1532 & 2556 & 3745 & 2652 & 3700 & 2624 \\
phase\_oracle\_13 & 14340 & 6140 & 10236 & 14955 & 10263 & 14922 & 10555 \\
phase\_oracle\_14 & 14340 & 6140 & 10236 & 14955 & 10263 & 14778 & 10502 \\
phase\_oracle\_5 & 52 & 20 & 36 & 61 & 45 & 64 & 45 \\
phase\_oracle\_6 & 52 & 20 & 36 & 61 & 45 & 61 & 45 \\
phase\_oracle\_7 & 222 & 92 & 156 & 252 & 165 & 249 & 167 \\
phase\_oracle\_8 & 222 & 92 & 156 & 252 & 165 & 249 & 167 \\
phase\_oracle\_9 & 896 & 380 & 636 & 986 & 660 & 968 & 668 \\
piecewise\_chebyshev\_11 & 9331 & 3520 & 7059 & 9814 & 7305 & 9844 & 7404 \\
piecewise\_chebyshev\_13 & 16649 & 6282 & 12639 & 17447 & 13184 & 17393 & 13147 \\
piecewise\_chebyshev\_15 & 27079 & 10218 & 20602 & 28285 & 21489 & 28432 & 21481 \\
piecewise\_chebyshev\_5 & 469 & 178 & 353 & 499 & 367 & 499 & 367 \\
piecewise\_chebyshev\_7 & 1799 & 678 & 1340 & 1925 & 1436 & 1925 & 1433 \\
piecewise\_chebyshev\_9 & 4567 & 1722 & 3435 & 4921 & 3678 & 4912 & 3663 \\
qft\_10 & 250 & 105 & 74 & 316 & 162 & 331 & 160 \\
qft\_11 & 301 & 125 & 82 & 394 & 210 & 394 & 210 \\
qft\_12 & 360 & 150 & 90 & 465 & 246 & 462 & 266 \\
qft\_13 & 421 & 174 & 98 & 559 & 329 & 562 & 339 \\
qft\_14 & 490 & 203 & 106 & 655 & 346 & 628 & 359 \\
qft\_15 & 561 & 231 & 114 & 738 & 373 & 762 & 340 \\
qft\_5 & 61 & 26 & 34 & 79 & 58 & 79 & 58 \\
qft\_6 & 90 & 39 & 42 & 114 & 85 & 123 & 83 \\
qft\_7 & 121 & 51 & 50 & 154 & 98 & 154 & 98 \\
qft\_8 & 160 & 68 & 58 & 202 & 134 & 202 & 134 \\
qft\_9 & 201 & 84 & 66 & 264 & 128 & 264 & 128 \\
quadratic\_form\_10 & 581 & 252 & 292 & 722 & 395 & 725 & 383 \\
quadratic\_form\_11 & 684 & 296 & 334 & 855 & 479 & 876 & 490 \\
quadratic\_form\_12 & 792 & 342 & 376 & 1005 & 580 & 975 & 594 \\
quadratic\_form\_13 & 905 & 390 & 418 & 1130 & 637 & 1130 & 637 \\
quadratic\_form\_14 & 1023 & 440 & 460 & 1266 & 738 & 1251 & 752 \\
quadratic\_form\_15 & 1146 & 492 & 502 & 1461 & 817 & 1455 & 809 \\
quadratic\_form\_5 & 141 & 62 & 82 & 165 & 109 & 165 & 109 \\
quadratic\_form\_6 & 219 & 96 & 124 & 264 & 169 & 264 & 169 \\
quadratic\_form\_7 & 302 & 132 & 166 & 362 & 210 & 362 & 210 \\
quadratic\_form\_8 & 390 & 170 & 208 & 477 & 286 & 468 & 274 \\
quadratic\_form\_9 & 483 & 210 & 250 & 606 & 374 & 615 & 366 \\
quantum\_volume\_10 & 550 & 150 & 70 & 613 & 176 & 613 & 176 \\
quantum\_volume\_11 & 605 & 165 & 77 & 701 & 248 & 701 & 248 \\
quantum\_volume\_12 & 792 & 216 & 84 & 921 & 269 & 915 & 299 \\
quantum\_volume\_13 & 858 & 234 & 91 & 990 & 331 & 993 & 351 \\
quantum\_volume\_14 & 1078 & 294 & 98 & 1246 & 398 & 1258 & 441 \\
quantum\_volume\_15 & 1155 & 315 & 105 & 1359 & 454 & 1356 & 458 \\
quantum\_volume\_5 & 110 & 30 & 35 & 125 & 50 & 128 & 48 \\
quantum\_volume\_6 & 198 & 54 & 42 & 222 & 77 & 222 & 77 \\
quantum\_volume\_7 & 231 & 63 & 49 & 255 & 106 & 255 & 106 \\
quantum\_volume\_8 & 352 & 96 & 56 & 388 & 143 & 388 & 143 \\
quantum\_volume\_9 & 396 & 108 & 63 & 447 & 156 & 447 & 156 \\
weighted\_adder\_12 & 863 & 319 & 571 & 1046 & 743 & 1046 & 749 \\
weighted\_adder\_15 & 1466 & 538 & 1003 & 1799 & 1263 & 1808 & 1280 \\
weighted\_adder\_6 & 96 & 38 & 63 & 114 & 69 & 114 & 69 \\
weighted\_adder\_9 & 367 & 137 & 229 & 463 & 300 & 451 & 279 \\
excitation\_preserving\_16 & 5104 & 1440 & 614 & 5701 & 2745 & 5758 & 2750 \\
excitation\_preserving\_17 & 5780 & 1632 & 654 & 6605 & 2911 & 6539 & 2698 \\
excitation\_preserving\_18 & 6498 & 1836 & 694 & 7371 & 3077 & 7329 & 3147 \\
excitation\_preserving\_19 & 7258 & 2052 & 734 & 8134 & 3243 & 8200 & 3522 \\
excitation\_preserving\_20 & 8060 & 2280 & 774 & 9149 & 3973 & 9179 & 4219 \\
hidden\_linear\_16 & 116 & 28 & 33 & 176 & 68 & 170 & 70 \\
hidden\_linear\_17 & 124 & 30 & 35 & 190 & 87 & 184 & 77 \\
hidden\_linear\_18 & 132 & 32 & 37 & 204 & 84 & 195 & 73 \\
hidden\_linear\_19 & 140 & 34 & 39 & 203 & 96 & 209 & 92 \\
hidden\_linear\_20 & 148 & 36 & 41 & 223 & 97 & 220 & 97 \\
inner\_product\_16 & 24 & 8 & 3 & 57 & 17 & 57 & 31 \\
inner\_product\_18 & 27 & 9 & 3 & 60 & 21 & 60 & 21 \\
inner\_product\_20 & 30 & 10 & 3 & 45 & 6 & 45 & 6 \\
integer\_comparator\_16 & 200 & 78 & 133 & 269 & 173 & 269 & 173 \\
integer\_comparator\_18 & 230 & 90 & 153 & 311 & 179 & 314 & 187 \\
integer\_comparator\_20 & 260 & 102 & 173 & 347 & 202 & 350 & 201 \\
IQP\_16 & 543 & 198 & 120 & 717 & 352 & 711 & 343 \\
IQP\_17 & 619 & 228 & 125 & 835 & 407 & 853 & 388 \\
IQP\_18 & 681 & 252 & 132 & 909 & 449 & 924 & 460 \\
IQP\_19 & 756 & 280 & 144 & 1005 & 478 & 1029 & 482 \\
IQP\_20 & 830 & 310 & 148 & 1115 & 493 & 1136 & 473 \\
piecewise\_chebyshev\_17 & 41179 & 15538 & 31375 & 43132 & 32720 & 43618 & 33075 \\
qft\_16 & 640 & 264 & 122 & 856 & 472 & 832 & 454 \\
qft\_17 & 721 & 296 & 130 & 964 & 479 & 952 & 485 \\
qft\_18 & 810 & 333 & 138 & 1104 & 502 & 1107 & 536 \\
qft\_19 & 901 & 369 & 146 & 1219 & 569 & 1267 & 638 \\
qft\_20 & 1000 & 410 & 154 & 1360 & 617 & 1375 & 658 \\
quadratic\_form\_16 & 1274 & 546 & 544 & 1667 & 949 & 1607 & 949 \\
quadratic\_form\_17 & 1407 & 602 & 586 & 1827 & 1021 & 1818 & 1026 \\
quadratic\_form\_18 & 1545 & 660 & 628 & 1998 & 1069 & 1962 & 1040 \\
quadratic\_form\_19 & 1688 & 720 & 670 & 2174 & 1213 & 2183 & 1229 \\
quadratic\_form\_20 & 1836 & 782 & 712 & 2400 & 1337 & 2361 & 1362 \\
quantum\_volume\_16 & 1408 & 384 & 112 & 1663 & 598 & 1663 & 547 \\
quantum\_volume\_17 & 1496 & 408 & 119 & 1802 & 519 & 1784 & 529 \\
quantum\_volume\_18 & 1782 & 486 & 126 & 2109 & 554 & 2118 & 641 \\
quantum\_volume\_19 & 1881 & 513 & 133 & 2223 & 668 & 2310 & 606 \\
quantum\_volume\_20 & 2200 & 600 & 140 & 2728 & 831 & 2701 & 836 \\
weighted\_adder\_18 & 2301 & 843 & 1592 & 2844 & 1972 & 2715 & 1944 \\
Summary & 603654 & 260589 & 413734 & 644664 & 455560 & 642261 & 462746\\
\hline

\end{longtable}

% Please add the following required packages to your document preamble:
% \usepackage{longtable}
% Note: It may be necessary to compile the document several times to get a multi-page table to line up properly
\begin{longtable}[c]{cccccccc}
\caption{Detailed results of MCTS-Depth and MCTS-Depth+r on IBM Q20 with naive initial mappings (Circuits are extracted from Qiskit library and each SWAP is decomposed into 3 CNOTs).}\\
\hline
\begin{tabular}[c]{@{}c@{}}Circuit\\      Name\end{tabular} & \begin{tabular}[c]{@{}c@{}}\#gate\\      input\end{tabular} & \begin{tabular}[c]{@{}c@{}}\#cnot\\    input  \end{tabular} & \begin{tabular}[c]{@{}c@{}}depth\\      input\end{tabular} & \begin{tabular}[c]{@{}c@{}}\#gate\\      mcts-d\end{tabular} & \begin{tabular}[c]{@{}c@{}}depth\\      mcts-d\end{tabular} & \begin{tabular}[c]{@{}c@{}}\#gate\\      mcts-d+r\end{tabular} & \begin{tabular}[c]{@{}c@{}}depth\\      mcts-d+r\end{tabular} \\
%\endfirsthead
%
\hline
\endhead
AND\_10 & 3067 & 1532 & 2556 & 3289 & 2585 & 3196 & 2597 \\
AND\_11 & 6139 & 3068 & 5116 & 6385 & 5143 & 6298 & 5193 \\
AND\_12 & 12283 & 6140 & 10236 & 12727 & 10260 & 12568 & 10373 \\
AND\_13 & 24571 & 12284 & 20476 & 25411 & 20506 & 25135 & 20738 \\
AND\_14 & 49147 & 24572 & 40956 & 50740 & 40989 & 50173 & 41583 \\
AND\_5 & 105 & 36 & 81 & 126 & 86 & 129 & 86 \\
AND\_6 & 187 & 92 & 156 & 217 & 168 & 223 & 165 \\
AND\_7 & 379 & 188 & 316 & 439 & 329 & 454 & 328 \\
AND\_8 & 763 & 380 & 636 & 868 & 645 & 883 & 651 \\
AND\_9 & 1531 & 764 & 1276 & 2026 & 1291 & 1648 & 1312 \\
excitation\_preserving\_10 & 1930 & 540 & 374 & 2302 & 732 & 2251 & 762 \\
excitation\_preserving\_11 & 2354 & 660 & 414 & 2831 & 915 & 2879 & 967 \\
excitation\_preserving\_12 & 2820 & 792 & 454 & 3441 & 1089 & 3591 & 1082 \\
excitation\_preserving\_13 & 3328 & 936 & 494 & 3958 & 1227 & 4276 & 1295 \\
excitation\_preserving\_14 & 3878 & 1092 & 534 & 4739 & 1387 & 4742 & 1500 \\
excitation\_preserving\_15 & 4470 & 1260 & 574 & 5457 & 1671 & 5295 & 1600 \\
excitation\_preserving\_5 & 440 & 120 & 174 & 512 & 240 & 521 & 212 \\
excitation\_preserving\_6 & 654 & 180 & 214 & 750 & 314 & 747 & 297 \\
excitation\_preserving\_7 & 910 & 252 & 254 & 1084 & 370 & 1105 & 407 \\
excitation\_preserving\_8 & 1208 & 336 & 294 & 1487 & 484 & 1427 & 494 \\
excitation\_preserving\_9 & 1548 & 432 & 334 & 1824 & 611 & 1941 & 631 \\
grover\_operator\_10 & 3110 & 1532 & 2562 & 3260 & 2589 & 3239 & 2603 \\
grover\_operator\_11 & 6186 & 3068 & 5122 & 6519 & 5149 & 6345 & 5199 \\
grover\_operator\_12 & 12334 & 6140 & 10242 & 12778 & 10267 & 12619 & 10379 \\
grover\_operator\_13 & 24626 & 12284 & 20482 & 26243 & 20501 & 25280 & 20746 \\
grover\_operator\_14 & 49206 & 24572 & 40962 & 50907 & 40996 & 50643 & 41864 \\
grover\_operator\_5 & 128 & 36 & 87 & 155 & 92 & 155 & 92 \\
grover\_operator\_6 & 214 & 92 & 162 & 244 & 173 & 244 & 173 \\
grover\_operator\_7 & 410 & 188 & 322 & 452 & 338 & 464 & 338 \\
grover\_operator\_8 & 798 & 380 & 642 & 903 & 653 & 882 & 656 \\
grover\_operator\_9 & 1570 & 764 & 1282 & 1693 & 1299 & 2245 & 1302 \\
hidden\_linear\_10 & 68 & 16 & 21 & 122 & 40 & 113 & 38 \\
hidden\_linear\_11 & 76 & 18 & 23 & 136 & 45 & 136 & 41 \\
hidden\_linear\_12 & 84 & 20 & 25 & 150 & 46 & 144 & 44 \\
hidden\_linear\_13 & 92 & 22 & 27 & 182 & 56 & 173 & 47 \\
hidden\_linear\_14 & 100 & 24 & 29 & 217 & 60 & 166 & 51 \\
hidden\_linear\_15 & 108 & 26 & 31 & 240 & 62 & 246 & 69 \\
hidden\_linear\_5 & 28 & 6 & 11 & 52 & 19 & 52 & 19 \\
hidden\_linear\_6 & 36 & 8 & 13 & 69 & 22 & 69 & 23 \\
hidden\_linear\_7 & 44 & 10 & 15 & 74 & 27 & 80 & 27 \\
hidden\_linear\_8 & 52 & 12 & 17 & 91 & 31 & 85 & 29 \\
hidden\_linear\_9 & 60 & 14 & 19 & 108 & 36 & 120 & 34 \\
inner\_product\_10 & 15 & 5 & 3 & 15 & 3 & 15 & 3 \\
inner\_product\_12 & 18 & 6 & 3 & 33 & 9 & 36 & 9 \\
inner\_product\_14 & 21 & 7 & 3 & 45 & 9 & 45 & 12 \\
inner\_product\_6 & 9 & 3 & 3 & 24 & 8 & 24 & 8 \\
inner\_product\_8 & 12 & 4 & 3 & 24 & 8 & 27 & 8 \\
integer\_comparator\_10 & 110 & 42 & 73 & 194 & 78 & 194 & 88 \\
integer\_comparator\_12 & 140 & 54 & 93 & 245 & 104 & 227 & 112 \\
integer\_comparator\_14 & 170 & 66 & 113 & 233 & 123 & 293 & 124 \\
integer\_comparator\_6 & 50 & 18 & 33 & 77 & 41 & 77 & 41 \\
integer\_comparator\_8 & 80 & 30 & 53 & 95 & 57 & 98 & 57 \\
IQP\_10 & 225 & 78 & 72 & 399 & 132 & 345 & 112 \\
IQP\_11 & 276 & 98 & 79 & 468 & 152 & 507 & 155 \\
IQP\_12 & 319 & 114 & 84 & 523 & 177 & 511 & 156 \\
IQP\_13 & 364 & 130 & 92 & 703 & 192 & 604 & 186 \\
IQP\_14 & 430 & 156 & 104 & 727 & 217 & 811 & 241 \\
IQP\_15 & 483 & 176 & 104 & 933 & 240 & 816 & 247 \\
IQP\_5 & 60 & 18 & 32 & 93 & 39 & 99 & 39 \\
IQP\_6 & 88 & 28 & 40 & 118 & 51 & 139 & 52 \\
IQP\_7 & 116 & 38 & 48 & 188 & 67 & 179 & 69 \\
IQP\_8 & 163 & 56 & 56 & 307 & 92 & 295 & 104 \\
IQP\_9 & 191 & 66 & 60 & 284 & 102 & 347 & 122 \\
OR\_10 & 3086 & 1532 & 2557 & 3449 & 2583 & 3215 & 2598 \\
OR\_11 & 6160 & 3068 & 5117 & 6406 & 5144 & 6319 & 5194 \\
OR\_12 & 12306 & 6140 & 10237 & 12750 & 10261 & 12591 & 10374 \\
OR\_13 & 24596 & 12284 & 20477 & 25703 & 20501 & 25070 & 20745 \\
OR\_14 & 49174 & 24572 & 40957 & 50767 & 40990 & 50611 & 41858 \\
OR\_5 & 114 & 36 & 82 & 138 & 87 & 138 & 87 \\
OR\_6 & 198 & 92 & 157 & 231 & 166 & 228 & 169 \\
OR\_7 & 392 & 188 & 317 & 449 & 327 & 446 & 334 \\
OR\_8 & 778 & 380 & 637 & 883 & 647 & 901 & 652 \\
OR\_9 & 1548 & 764 & 1277 & 1812 & 1293 & 1668 & 1313 \\
phase\_estimation\_10 & 3981 & 1586 & 2604 & 4134 & 2662 & 4095 & 2642 \\
phase\_estimation\_11 & 7863 & 3138 & 5172 & 7989 & 5226 & 8007 & 5237 \\
phase\_estimation\_12 & 15590 & 6228 & 10300 & 15770 & 10367 & 15743 & 10374 \\
phase\_estimation\_13 & 31002 & 12392 & 20548 & 31254 & 20653 & 31215 & 20642 \\
phase\_estimation\_5 & 126 & 48 & 84 & 159 & 93 & 162 & 94 \\
phase\_estimation\_6 & 263 & 102 & 172 & 299 & 189 & 299 & 189 \\
phase\_estimation\_7 & 525 & 206 & 340 & 600 & 367 & 573 & 355 \\
phase\_estimation\_8 & 1032 & 408 & 668 & 1143 & 697 & 1107 & 690 \\
phase\_estimation\_9 & 2024 & 804 & 1316 & 2141 & 1357 & 2141 & 1358 \\
phase\_oracle\_10 & 896 & 380 & 636 & 956 & 648 & 947 & 654 \\
phase\_oracle\_11 & 3586 & 1532 & 2556 & 3730 & 2582 & 3700 & 2610 \\
phase\_oracle\_12 & 3586 & 1532 & 2556 & 3739 & 2571 & 3700 & 2607 \\
phase\_oracle\_13 & 14340 & 6140 & 10236 & 14916 & 10260 & 14676 & 10371 \\
phase\_oracle\_14 & 14340 & 6140 & 10236 & 14916 & 10260 & 14649 & 10381 \\
phase\_oracle\_5 & 52 & 20 & 36 & 70 & 39 & 70 & 39 \\
phase\_oracle\_6 & 52 & 20 & 36 & 70 & 39 & 70 & 39 \\
phase\_oracle\_7 & 222 & 92 & 156 & 255 & 162 & 255 & 162 \\
phase\_oracle\_8 & 222 & 92 & 156 & 255 & 162 & 255 & 162 \\
phase\_oracle\_9 & 896 & 380 & 636 & 956 & 648 & 947 & 654 \\
piecewise\_chebyshev\_11 & 9331 & 3520 & 7059 & 9898 & 7202 & 9991 & 7198 \\
piecewise\_chebyshev\_13 & 16649 & 6282 & 12639 & 17744 & 12948 & 17702 & 12921 \\
piecewise\_chebyshev\_15 & 27079 & 10218 & 20602 & 28774 & 21092 & 28459 & 20982 \\
piecewise\_chebyshev\_5 & 469 & 178 & 353 & 514 & 356 & 520 & 359 \\
piecewise\_chebyshev\_7 & 1799 & 678 & 1340 & 1961 & 1371 & 1964 & 1374 \\
piecewise\_chebyshev\_9 & 4567 & 1722 & 3435 & 4924 & 3508 & 4990 & 3513 \\
qft\_10 & 250 & 105 & 74 & 397 & 127 & 388 & 122 \\
qft\_11 & 301 & 125 & 82 & 481 & 157 & 574 & 177 \\
qft\_12 & 360 & 150 & 90 & 705 & 192 & 669 & 196 \\
qft\_13 & 421 & 174 & 98 & 865 & 229 & 685 & 216 \\
qft\_14 & 490 & 203 & 106 & 871 & 231 & 994 & 257 \\
qft\_15 & 561 & 231 & 114 & 897 & 278 & 1008 & 282 \\
qft\_5 & 61 & 26 & 34 & 109 & 44 & 112 & 44 \\
qft\_6 & 90 & 39 & 42 & 135 & 59 & 159 & 69 \\
qft\_7 & 121 & 51 & 50 & 193 & 77 & 163 & 76 \\
qft\_8 & 160 & 68 & 58 & 280 & 101 & 265 & 94 \\
qft\_9 & 201 & 84 & 66 & 366 & 125 & 297 & 120 \\
quadratic\_form\_10 & 581 & 252 & 292 & 896 & 362 & 827 & 368 \\
quadratic\_form\_11 & 684 & 296 & 334 & 1014 & 451 & 1050 & 445 \\
quadratic\_form\_12 & 792 & 342 & 376 & 1251 & 528 & 1185 & 504 \\
quadratic\_form\_13 & 905 & 390 & 418 & 1370 & 580 & 1358 & 551 \\
quadratic\_form\_14 & 1023 & 440 & 460 & 1626 & 620 & 1578 & 622 \\
quadratic\_form\_15 & 1146 & 492 & 502 & 1812 & 708 & 1812 & 720 \\
quadratic\_form\_5 & 141 & 62 & 82 & 189 & 100 & 186 & 93 \\
quadratic\_form\_6 & 219 & 96 & 124 & 348 & 145 & 297 & 140 \\
quadratic\_form\_7 & 302 & 132 & 166 & 404 & 200 & 404 & 193 \\
quadratic\_form\_8 & 390 & 170 & 208 & 543 & 253 & 531 & 250 \\
quadratic\_form\_9 & 483 & 210 & 250 & 741 & 313 & 840 & 331 \\
quantum\_volume\_10 & 550 & 150 & 70 & 703 & 165 & 748 & 181 \\
quantum\_volume\_11 & 605 & 165 & 77 & 815 & 206 & 815 & 209 \\
quantum\_volume\_12 & 792 & 216 & 84 & 1074 & 248 & 1140 & 272 \\
quantum\_volume\_13 & 858 & 234 & 91 & 1173 & 285 & 1170 & 285 \\
quantum\_volume\_14 & 1078 & 294 & 98 & 1447 & 343 & 1492 & 370 \\
quantum\_volume\_15 & 1155 & 315 & 105 & 1575 & 356 & 1611 & 391 \\
quantum\_volume\_5 & 110 & 30 & 35 & 155 & 50 & 152 & 50 \\
quantum\_volume\_6 & 198 & 54 & 42 & 240 & 74 & 303 & 81 \\
quantum\_volume\_7 & 231 & 63 & 49 & 282 & 104 & 288 & 79 \\
quantum\_volume\_8 & 352 & 96 & 56 & 433 & 111 & 478 & 158 \\
quantum\_volume\_9 & 396 & 108 & 63 & 480 & 124 & 489 & 156 \\
weighted\_adder\_12 & 863 & 319 & 571 & 1247 & 646 & 1175 & 619 \\
weighted\_adder\_15 & 1466 & 538 & 1003 & 2072 & 1129 & 2093 & 1121 \\
weighted\_adder\_6 & 96 & 38 & 63 & 114 & 69 & 114 & 69 \\
weighted\_adder\_9 & 367 & 137 & 229 & 529 & 263 & 526 & 254 \\
excitation\_preserving\_16 & 5104 & 1440 & 614 & 6376 & 1849 & 6433 & 1933 \\
excitation\_preserving\_17 & 5780 & 1632 & 654 & 7034 & 2089 & 7316 & 2121 \\
excitation\_preserving\_18 & 6498 & 1836 & 694 & 8295 & 2423 & 8037 & 2360 \\
excitation\_preserving\_19 & 7258 & 2052 & 734 & 9361 & 2738 & 9118 & 2548 \\
excitation\_preserving\_20 & 8060 & 2280 & 774 & 10235 & 2747 & 10619 & 2968 \\
hidden\_linear\_16 & 116 & 28 & 33 & 236 & 68 & 218 & 64 \\
hidden\_linear\_17 & 124 & 30 & 35 & 259 & 69 & 244 & 70 \\
hidden\_linear\_18 & 132 & 32 & 37 & 243 & 78 & 222 & 69 \\
hidden\_linear\_19 & 140 & 34 & 39 & 263 & 76 & 257 & 81 \\
hidden\_linear\_20 & 148 & 36 & 41 & 322 & 86 & 286 & 83 \\
inner\_product\_16 & 24 & 8 & 3 & 72 & 14 & 84 & 14 \\
inner\_product\_18 & 27 & 9 & 3 & 105 & 17 & 90 & 17 \\
inner\_product\_20 & 30 & 10 & 3 & 60 & 12 & 54 & 10 \\
integer\_comparator\_16 & 200 & 78 & 133 & 383 & 154 & 344 & 155 \\
integer\_comparator\_18 & 230 & 90 & 153 & 386 & 159 & 422 & 165 \\
integer\_comparator\_20 & 260 & 102 & 173 & 473 & 195 & 416 & 187 \\
IQP\_16 & 543 & 198 & 120 & 957 & 289 & 996 & 296 \\
IQP\_17 & 619 & 228 & 125 & 1135 & 319 & 1144 & 315 \\
IQP\_18 & 681 & 252 & 132 & 1365 & 345 & 1284 & 339 \\
IQP\_19 & 756 & 280 & 144 & 1362 & 374 & 1347 & 381 \\
IQP\_20 & 830 & 310 & 148 & 1409 & 389 & 1451 & 374 \\
piecewise\_chebyshev\_17 & 41179 & 15538 & 31375 & 43504 & 32032 & 43387 & 32055 \\
qft\_16 & 640 & 264 & 122 & 1108 & 330 & 1141 & 334 \\
qft\_17 & 721 & 296 & 130 & 1297 & 373 & 1348 & 382 \\
qft\_18 & 810 & 333 & 138 & 1416 & 407 & 1632 & 441 \\
qft\_19 & 901 & 369 & 146 & 1582 & 439 & 1534 & 420 \\
qft\_20 & 1000 & 410 & 154 & 1828 & 478 & 1816 & 485 \\
quadratic\_form\_16 & 1274 & 546 & 544 & 1928 & 791 & 2120 & 771 \\
quadratic\_form\_17 & 1407 & 602 & 586 & 2385 & 873 & 2199 & 825 \\
quadratic\_form\_18 & 1545 & 660 & 628 & 2550 & 953 & 2487 & 941 \\
quadratic\_form\_19 & 1688 & 720 & 670 & 2846 & 1045 & 2756 & 1012 \\
quadratic\_form\_20 & 1836 & 782 & 712 & 3141 & 1132 & 3015 & 1105 \\
quantum\_volume\_16 & 1408 & 384 & 112 & 1951 & 472 & 1927 & 460 \\
quantum\_volume\_17 & 1496 & 408 & 119 & 2114 & 489 & 2249 & 542 \\
quantum\_volume\_18 & 1782 & 486 & 126 & 2601 & 583 & 2499 & 547 \\
quantum\_volume\_19 & 1881 & 513 & 133 & 2721 & 586 & 2691 & 541 \\
quantum\_volume\_20 & 2200 & 600 & 140 & 3424 & 749 & 3394 & 755 \\
weighted\_adder\_18 & 2301 & 843 & 1592 & 3396 & 1794 & 3339 & 1780 \\
Summary & 603654 & 260589 & 413734 & 668646 & 440971 & 663987 & 445034 \\
\hline
\end{longtable}
