# Supplementary material for: Quantum Circuit Transformation: A Monte Carlo Tree Search Framework
Source: arXiv:2008.09331 source file (2022-01-25)
Supplement: Supplementary file 2 [file appendix_old.tex]

\onecolumn


% \begin{table}[]
% 	\centering
% 	\caption{Comparison of MCTS-Size with SAHS \cite{SAHS} on IBM Q20.}
% 	\label{tab:SAHS_Q20_small}
% 	\begin{tabular}{ccccc}
% 		\hline
% 		\begin{tabular}[c]{@{}c@{}}Circuit\\      Name\end{tabular} & \begin{tabular}[c]{@{}c@{}}Input\\      CNOT\end{tabular} & \begin{tabular}[c]{@{}c@{}}Added\\       SAHS\end{tabular} & \begin{tabular}[c]{@{}c@{}}Added\\      MCTS-Size\end{tabular} & Improvement \\
% 		\hline
% 		rd84\_142 & 154 & 102 & 66 & 35.29\% \\
% 		adr4\_197 & 1498 & 711 & 414 & 41.77\% \\
% 		radd\_250 & 1405 & 729 & 471 & 35.39\% \\
% 		z4\_268 & 1343 & 546 & 390 & 28.57\% \\
% 		sym6\_145 & 1701 & 744 & 339 & 54.44\% \\
% 		misex1\_241 & 2100 & 921 & 357 & 61.24\% \\
% 		rd73\_252 & 2319 & 1125 & 783 & 30.40\% \\
% 		cycle10\_2\_110 & 2648 & 1038 & 738 & 28.90\% \\
% 		square\_root\_7 & 3089 & 1353 & 624 & 53.88\% \\
% 		sqn\_258 & 4459 & 1953 & 1182 & 39.48\% \\
% 		rd84\_253 & 5960 & 3198 & 1881 & 41.18\% \\
% 		Summary & 26676 & 12420 & 7245 & 41.67\% \\
% 		\hline
% 	\end{tabular}
% \end{table}

\section{Large Circuit Set Benchmarks Compared to SAHS}
% Please add the following required packages to your document preamble:
% \usepackage{longtable}
% Note: It may be necessary to compile the document several times to get a multi-page table to line up properly
\begin{longtable}[c]{ccccc}
\caption{Comparison of MCTS-Size with SAHS \cite{SAHS} on IBM Q20.}
\label{tab:SAHS_Q20}\\
%\\
\hline
\begin{tabular}[c]{@{}c@{}}Circuit\\      Name\end{tabular} & \begin{tabular}[c]{@{}c@{}}Input\\      CNOT\end{tabular} & \begin{tabular}[c]{@{}c@{}}CNOT Added\\       SAHS\end{tabular} & \begin{tabular}[c]{@{}c@{}}CNOT Added\\      MCTS-Size\end{tabular} & Improvement \\
\hline
\endhead
%
graycode6\_47 & 5 & 0 & 0 & 0.0\% \\
xor5\_254 & 5 & 0 & 0 & 0.0\% \\
ex1\_226 & 5 & 0 & 0 & 0.0\% \\
4gt11\_84 & 9 & 0 & 0 & 0.0\% \\
ex-1\_166 & 9 & 0 & 0 & 0.0\% \\
ham3\_102 & 11 & 0 & 0 & 0.0\% \\
4mod5-v0\_20 & 10 & 0 & 0 & 0.0\% \\
4mod5-v1\_22 & 11 & 0 & 0 & 0.0\% \\
mod5d1\_63 & 13 & 0 & 0 & 0.0\% \\
4gt11\_83 & 14 & 0 & 0 & 0.0\% \\
4gt11\_82 & 18 & 3 & 3 & 0.0\% \\
rd32-v0\_66 & 16 & 0 & 0 & 0.0\% \\
mod5mils\_65 & 16 & 0 & 0 & 0.0\% \\
4mod5-v0\_19 & 16 & 0 & 0 & 0.0\% \\
rd32-v1\_68 & 16 & 0 & 0 & 0.0\% \\
alu-v0\_27 & 17 & 6 & 6 & 0.0\% \\
3\_17\_13 & 17 & 0 & 0 & 0.0\% \\
4mod5-v1\_24 & 16 & 0 & 0 & 0.0\% \\
alu-v1\_29 & 17 & 6 & 6 & 0.0\% \\
alu-v1\_28 & 18 & 6 & 6 & 0.0\% \\
alu-v3\_35 & 18 & 6 & 6 & 0.0\% \\
alu-v2\_33 & 17 & 6 & 6 & 0.0\% \\
alu-v4\_37 & 18 & 6 & 6 & 0.0\% \\
miller\_11 & 23 & 0 & 0 & 0.0\% \\
decod24-v0\_38 & 23 & 0 & 0 & 0.0\% \\
alu-v3\_34 & 24 & 6 & 6 & 0.0\% \\
decod24-v2\_43 & 22 & 0 & 0 & 0.0\% \\
mod5d2\_64 & 25 & 12 & 12 & 0.0\% \\
4gt13\_92 & 30 & 0 & 0 & 0.0\% \\
4gt13-v1\_93 & 30 & 0 & 0 & 0.0\% \\
one-two-three-v2\_100 & 32 & 9 & 9 & 0.0\% \\
4mod5-v1\_23 & 32 & 9 & 9 & 0.0\% \\
4mod5-v0\_18 & 31 & 9 & 9 & 0.0\% \\
one-two-three-v3\_101 & 32 & 6 & 6 & 0.0\% \\
4mod5-bdd\_287 & 31 & 6 & 6 & 0.0\% \\
decod24-bdd\_294 & 32 & 15 & 15 & 0.0\% \\
4gt5\_75 & 38 & 15 & 15 & 0.0\% \\
alu-v0\_26 & 38 & 9 & 9 & 0.0\% \\
rd32\_270 & 36 & 12 & 12 & 0.0\% \\
alu-bdd\_288 & 38 & 24 & 15 & 37.5\% \\
decod24-v1\_41 & 38 & 15 & 12 & 20.0\% \\
4gt5\_76 & 46 & 15 & 15 & 0.0\% \\
4gt13\_91 & 49 & 15 & 15 & 0.0\% \\
4gt13\_90 & 53 & 27 & 21 & 22.2\% \\
alu-v4\_36 & 51 & 15 & 15 & 0.0\% \\
4gt5\_77 & 58 & 9 & 9 & 0.0\% \\
one-two-three-v1\_99 & 59 & 12 & 12 & 0.0\% \\
rd53\_138 & 60 & 27 & 27 & 0.0\% \\
one-two-three-v0\_98 & 65 & 24 & 24 & 0.0\% \\
4gt10-v1\_81 & 66 & 27 & 21 & 22.2\% \\
decod24-v3\_45 & 64 & 15 & 15 & 0.0\% \\
aj-e11\_165 & 69 & 18 & 18 & 0.0\% \\
4mod7-v0\_94 & 72 & 12 & 12 & 0.0\% \\
alu-v2\_32 & 72 & 15 & 15 & 0.0\% \\
4mod7-v1\_96 & 72 & 18 & 18 & 0.0\% \\
cnt3-5\_179 & 85 & 15 & 9 & 40.0\% \\
mod10\_176 & 78 & 24 & 24 & 0.0\% \\
4gt4-v0\_80 & 79 & 24 & 24 & 0.0\% \\
4gt12-v0\_88 & 86 & 21 & 21 & 0.0\% \\
0410184\_169 & 104 & 12 & 12 & 0.0\% \\
4\_49\_16 & 99 & 36 & 27 & 25.0\% \\
4gt12-v1\_89 & 100 & 24 & 15 & 37.5\% \\
4gt4-v0\_79 & 105 & 12 & 9 & 25.0\% \\
hwb4\_49 & 107 & 33 & 30 & 9.1\% \\
4gt4-v0\_78 & 109 & 15 & 15 & 0.0\% \\
mod10\_171 & 108 & 24 & 24 & 0.0\% \\
4gt12-v0\_87 & 112 & 6 & 6 & 0.0\% \\
4gt12-v0\_86 & 116 & 9 & 9 & 0.0\% \\
4gt4-v0\_72 & 113 & 42 & 18 & 57.1\% \\
4gt4-v1\_74 & 119 & 78 & 30 & 61.5\% \\
mini-alu\_167 & 126 & 33 & 33 & 0.0\% \\
one-two-three-v0\_97 & 128 & 66 & 39 & 40.9\% \\
rd53\_135 & 134 & 54 & 54 & 0.0\% \\
ham7\_104 & 149 & 81 & 60 & 25.9\% \\
decod24-enable\_126 & 149 & 87 & 54 & 37.9\% \\
mod8-10\_178 & 152 & 21 & 21 & 0.0\% \\
4gt4-v0\_73 & 179 & 42 & 42 & 0.0\% \\
ex3\_229 & 175 & 18 & 18 & 0.0\% \\
mod8-10\_177 & 196 & 39 & 36 & 7.7\% \\
alu-v2\_31 & 198 & 54 & 48 & 11.1\% \\
C17\_204 & 205 & 96 & 60 & 37.5\% \\
rd53\_131 & 200 & 90 & 51 & 43.3\% \\
alu-v2\_30 & 223 & 45 & 45 & 0.0\% \\
mod5adder\_127 & 239 & 51 & 51 & 0.0\% \\
rd53\_133 & 256 & 105 & 84 & 20.0\% \\
majority\_239 & 267 & 84 & 60 & 28.6\% \\
ex2\_227 & 275 & 96 & 78 & 18.7\% \\
cm82a\_208 & 283 & 84 & 84 & 0.0\% \\
sf\_276 & 336 & 24 & 24 & 0.0\% \\
sf\_274 & 336 & 24 & 24 & 0.0\% \\
con1\_216 & 415 & 192 & 102 & 46.9\% \\
rd53\_130 & 448 & 171 & 132 & 22.8\% \\
f2\_232 & 525 & 213 & 105 & 50.7\% \\
rd53\_251 & 564 & 204 & 147 & 27.9\% \\
hwb5\_53 & 598 & 174 & 159 & 8.6\% \\
radd\_250 & 1405 & 669 & 441 & 34.1\% \\
rd73\_252 & 2319 & 1065 & 627 & 41.1\% \\
cycle10\_2\_110 & 2648 & 1296 & 759 & 41.4\% \\
hwb6\_56 & 2952 & 1104 & 813 & 26.4\% \\
cm85a\_209 & 4986 & 2337 & 1278 & 45.3\% \\
rd84\_253 & 5960 & 3246 & 1950 & 39.9\% \\
root\_255 & 7493 & 3525 & 2082 & 40.9\% \\
mlp4\_245 & 8232 & 4116 & 2670 & 35.1\% \\
urf2\_277 & 10066 & 5934 & 4470 & 24.7\% \\
sym9\_148 & 9408 & 2172 & 1146 & 47.2\% \\
hwb7\_59 & 10681 & 4602 & 2769 & 39.8\% \\
clip\_206 & 14772 & 6843 & 4596 & 32.8\% \\
sym9\_193 & 15232 & 6441 & 4104 & 36.3\% \\
dist\_223 & 16624 & 6936 & 4719 & 32.0\% \\
sao2\_257 & 16864 & 7827 & 4515 & 42.3\% \\
urf5\_280 & 23764 & 13065 & 8721 & 33.2\% \\
urf1\_278 & 26692 & 15678 & 11040 & 29.6\% \\
sym10\_262 & 28084 & 11697 & 6636 & 43.3\% \\
hwb8\_113 & 30372 & 14976 & 8127 & 45.7\% \\
summary & 248553 & 116487 & 73758 & 36.7\% \\
\hline
\end{longtable}

\section{More Initial Mappings}
%Comparison of our algorithm based on various initial mappings, Naive, Topgraph (Topg.) \cite{SubgraphIsomorphism} and Weightedgraph (Weightg.) \cite{SubgraphIsomorphism}, with that in \cite{SAHS} on IBM Q20.

% Please add the following required packages to your document preamble:
% \usepackage{longtable}
% Note: It may be necessary to compile the document several times to get a multi-page table to line up properly
\begin{longtable}[c]{cccccccc}
\caption{Comparison of MCTS-Size to  FiDLS \cite{SubgraphIsomorphism} based on various initial mappings including Naive, Topgraph (topgr.) \cite{SubgraphIsomorphism} and Weighted graph (wgtgr.) \cite{SubgraphIsomorphism} on IBM Q20.}
%\label{tab:initial_mappings}\\
\\
\hline
\begin{tabular}[c]{@{}c@{}} \small Circuit\\      Name\end{tabular} & \begin{tabular}[c]{@{}c@{}}Input\\      CNOT\end{tabular} & \begin{tabular}[c]{@{}c@{}} \small CNOT Added\\    \small  Naive MCTS\end{tabular} & \begin{tabular}[c]{@{}c@{}} \small CNOT Added\\   \small     Topg. FiDLS\end{tabular} & \begin{tabular}[c]{@{}c@{}}  \small CNOT Added\\   \small     Topg. MCTS\end{tabular} & \begin{tabular}[c]{@{}c@{}}  \small CNOT Added\\    \small    Weig. FiDLS\end{tabular} & \begin{tabular}[c]{@{}c@{}}  \small CNOT Added\\    \small    Topg. MCTS\end{tabular} \\
\hline
\endhead
%
graycode6\_47 & 5 & 9 & 0 & 0 & 0 & 0 \\
xor5\_254 & 5 & 15 & 0 & 0 & 0 & 0 \\
ex1\_226 & 5 & 15 & 0 & 0 & 0 & 0 \\
4gt11\_84 & 9 & 12 & 0 & 0 & 0 & 0 \\
ex-1\_166 & 9 & 6 & 0 & 0 & 0 & 0 \\
ham3\_102 & 11 & 6 & 0 & 0 & 0 & 0 \\
4mod5-v0\_20 & 10 & 9 & 0 & 0 & 0 & 0 \\
4mod5-v1\_22 & 11 & 9 & 0 & 0 & 0 & 0 \\
mod5d1\_63 & 13 & 12 & 0 & 0 & 0 & 0 \\
4gt11\_83 & 14 & 12 & 0 & 0 & 0 & 0 \\
4gt11\_82 & 18 & 15 & 3 & 3 & 3 & 3 \\
rd32-v0\_66 & 16 & 12 & 0 & 0 & 0 & 0 \\
mod5mils\_65 & 16 & 18 & 0 & 0 & 0 & 0 \\
4mod5-v0\_19 & 16 & 15 & 0 & 0 & 0 & 0 \\
rd32-v1\_68 & 16 & 12 & 0 & 0 & 0 & 0 \\
alu-v0\_27 & 17 & 15 & 9 & 6 & 6 & 9 \\
3\_17\_13 & 17 & 6 & 0 & 0 & 0 & 0 \\
4mod5-v1\_24 & 16 & 15 & 0 & 0 & 0 & 0 \\
alu-v1\_29 & 17 & 18 & 9 & 6 & 6 & 9 \\
alu-v1\_28 & 18 & 15 & 9 & 6 & 6 & 9 \\
alu-v3\_35 & 18 & 15 & 9 & 6 & 6 & 9 \\
alu-v2\_33 & 17 & 15 & 9 & 6 & 6 & 6 \\
alu-v4\_37 & 18 & 15 & 9 & 6 & 6 & 9 \\
miller\_11 & 23 & 6 & 0 & 0 & 0 & 0 \\
decod24-v0\_38 & 23 & 12 & 0 & 0 & 0 & 0 \\
alu-v3\_34 & 24 & 15 & 9 & 6 & 6 & 12 \\
decod24-v2\_43 & 22 & 12 & 0 & 0 & 0 & 0 \\
mod5d2\_64 & 25 & 21 & 18 & 9 & 9 & 12 \\
4gt13\_92 & 30 & 21 & 0 & 0 & 0 & 0 \\
4gt13-v1\_93 & 30 & 24 & 0 & 0 & 0 & 0 \\
one-two-three-v2\_100 & 32 & 24 & 9 & 9 & 9 & 9 \\
4mod5-v1\_23 & 32 & 24 & 9 & 15 & 21 & 9 \\
4mod5-v0\_18 & 31 & 24 & 9 & 12 & 12 & 9 \\
one-two-three-v3\_101 & 32 & 27 & 15 & 9 & 18 & 9 \\
4mod5-bdd\_287 & 31 & 21 & 6 & 12 & 18 & 6 \\
decod24-bdd\_294 & 32 & 21 & 15 & 15 & 27 & 12 \\
4gt5\_75 & 38 & 24 & 9 & 9 & 12 & 15 \\
alu-v0\_26 & 38 & 27 & 12 & 9 & 9 & 12 \\
rd32\_270 & 36 & 27 & 18 & 18 & 24 & 12 \\
alu-bdd\_288 & 38 & 27 & 24 & 15 & 15 & 24 \\
decod24-v1\_41 & 38 & 30 & 3 & 15 & 21 & 3 \\
4gt5\_76 & 46 & 27 & 21 & 24 & 36 & 15 \\
4gt13\_91 & 49 & 27 & 6 & 6 & 6 & 6 \\
4gt13\_90 & 53 & 30 & 9 & 9 & 9 & 9 \\
alu-v4\_36 & 51 & 30 & 6 & 21 & 15 & 6 \\
4gt5\_77 & 58 & 24 & 9 & 18 & 18 & 9 \\
one-two-three-v1\_99 & 59 & 30 & 24 & 27 & 33 & 15 \\
rd53\_138 & 60 & 33 & 30 & 30 & 42 & 24 \\
one-two-three-v0\_98 & 65 & 39 & 18 & 27 & 27 & 18 \\
4gt10-v1\_81 & 66 & 33 & 15 & 18 & 18 & 15 \\
decod24-v3\_45 & 64 & 39 & 15 & 24 & 24 & 15 \\
aj-e11\_165 & 69 & 33 & 33 & 21 & 36 & 18 \\
4mod7-v0\_94 & 72 & 42 & 12 & 27 & 27 & 12 \\
alu-v2\_32 & 72 & 27 & 15 & 21 & 45 & 15 \\
4mod7-v1\_96 & 72 & 33 & 21 & 21 & 21 & 27 \\
cnt3-5\_179 & 85 & 63 & 3 & 15 & 30 & 3 \\
mod10\_176 & 78 & 36 & 15 & 24 & 24 & 15 \\
4gt4-v0\_80 & 79 & 48 & 15 & 12 & 39 & 21 \\
4gt12-v0\_88 & 86 & 48 & 21 & 12 & 15 & 18 \\
0410184\_169 & 104 & 72 & 6 & 24 & 27 & 6 \\
4\_49\_16 & 99 & 42 & 18 & 30 & 30 & 21 \\
4gt12-v1\_89 & 100 & 36 & 57 & 12 & 18 & 27 \\
4gt4-v0\_79 & 105 & 54 & 12 & 9 & 12 & 9 \\
hwb4\_49 & 107 & 42 & 36 & 39 & 42 & 30 \\
4gt4-v0\_78 & 109 & 60 & 15 & 15 & 15 & 15 \\
mod10\_171 & 108 & 42 & 39 & 27 & 27 & 33 \\
4gt12-v0\_87 & 112 & 60 & 6 & 6 & 6 & 6 \\
4gt12-v0\_86 & 116 & 63 & 9 & 9 & 9 & 9 \\
4gt4-v0\_72 & 113 & 60 & 45 & 36 & 39 & 27 \\
4gt4-v1\_74 & 119 & 72 & 39 & 27 & 27 & 24 \\
mini-alu\_167 & 126 & 48 & 30 & 33 & 33 & 30 \\
one-two-three-v0\_97 & 128 & 57 & 42 & 51 & 78 & 36 \\
rd53\_135 & 134 & 81 & 60 & 66 & 84 & 60 \\
ham7\_104 & 149 & 51 & 48 & 39 & 42 & 36 \\
decod24-enable\_126 & 149 & 69 & 66 & 51 & 63 & 42 \\
mod8-10\_178 & 152 & 33 & 69 & 24 & 33 & 48 \\
4gt4-v0\_73 & 179 & 66 & 99 & 42 & 42 & 87 \\
ex3\_229 & 175 & 42 & 24 & 24 & 81 & 15 \\
mod8-10\_177 & 196 & 57 & 123 & 42 & 78 & 54 \\
alu-v2\_31 & 198 & 81 & 78 & 60 & 90 & 57 \\
C17\_204 & 205 & 81 & 111 & 72 & 84 & 63 \\
rd53\_131 & 200 & 78 & 63 & 75 & 78 & 33 \\
alu-v2\_30 & 223 & 84 & 60 & 57 & 54 & 51 \\
mod5adder\_127 & 239 & 69 & 84 & 51 & 81 & 81 \\
rd53\_133 & 256 & 84 & 60 & 90 & 174 & 39 \\
majority\_239 & 267 & 96 & 66 & 84 & 105 & 93 \\
ex2\_227 & 275 & 93 & 78 & 90 & 108 & 72 \\
cm82a\_208 & 283 & 93 & 117 & 78 & 105 & 60 \\
sf\_276 & 336 & 60 & 36 & 24 & 36 & 24 \\
sf\_274 & 336 & 45 & 30 & 24 & 36 & 69 \\
con1\_216 & 415 & 138 & 273 & 111 & 153 & 162 \\
rd53\_130 & 448 & 126 & 267 & 144 & 207 & 129 \\
f2\_232 & 525 & 114 & 336 & 111 & 126 & 117 \\
rd53\_251 & 564 & 159 & 201 & 144 & 195 & 165 \\
hwb5\_53 & 598 & 174 & 207 & 171 & 204 & 156 \\
radd\_250 & 1405 & 453 & 633 & 474 & 567 & 435 \\
rd73\_252 & 2319 & 813 & 1062 & 630 & 852 & 825 \\
cycle10\_2\_110 & 2648 & 891 & 1125 & 954 & 1290 & 912 \\
hwb6\_56 & 2952 & 825 & 1077 & 783 & 1026 & 834 \\
cm85a\_209 & 4986 & 1479 & 2073 & 1449 & 2091 & 1140 \\
rd84\_253 & 5960 & 1959 & 2952 & 1995 & 2841 & 2055 \\
root\_255 & 7493 & 2442 & 2928 & 2196 & 3099 & 2013 \\
mlp4\_245 & 8232 & 2811 & 4275 & 2838 & 4146 & 2844 \\
urf2\_277 & 10066 & 4551 & 6285 & 4605 & 6267 & 4560 \\
sym9\_148 & 9408 & 1206 & 1947 & 1311 & 2166 & 1131 \\
hwb7\_59 & 10681 & 2826 & 3684 & 2904 & 3846 & 2805 \\
clip\_206 & 14772 & 4773 & 6762 & 4677 & 6834 & 4764 \\
sym9\_193 & 15232 & 3783 & 5481 & 3855 & 6462 & 4020 \\
dist\_223 & 16624 & 4560 & 7470 & 4764 & 6582 & 4857 \\
sao2\_257 & 16864 & 4899 & 7596 & 4386 & 6756 & 4749 \\
urf5\_280 & 23764 & 8721 & 11988 & 8946 & 11679 & 8916 \\
urf1\_278 & 26692 & 10824 & 13872 & 10749 & 13809 & 10548 \\
sym10\_262 & 28084 & 7500 & 11490 & 6633 & 10623 & 7284 \\
hwb8\_113 & 30372 & 8226 & 11295 & 8073 & 11382 & 7989 \\
Summary & 248553 & 77544 & 107406 & 74763 & 105645 & 75126 \\
\hline
\end{longtable}

\section{MCTS Depth Analysis}
\begin{figure}[ht]
	\centering
	\includegraphics[width=0.7\textwidth]{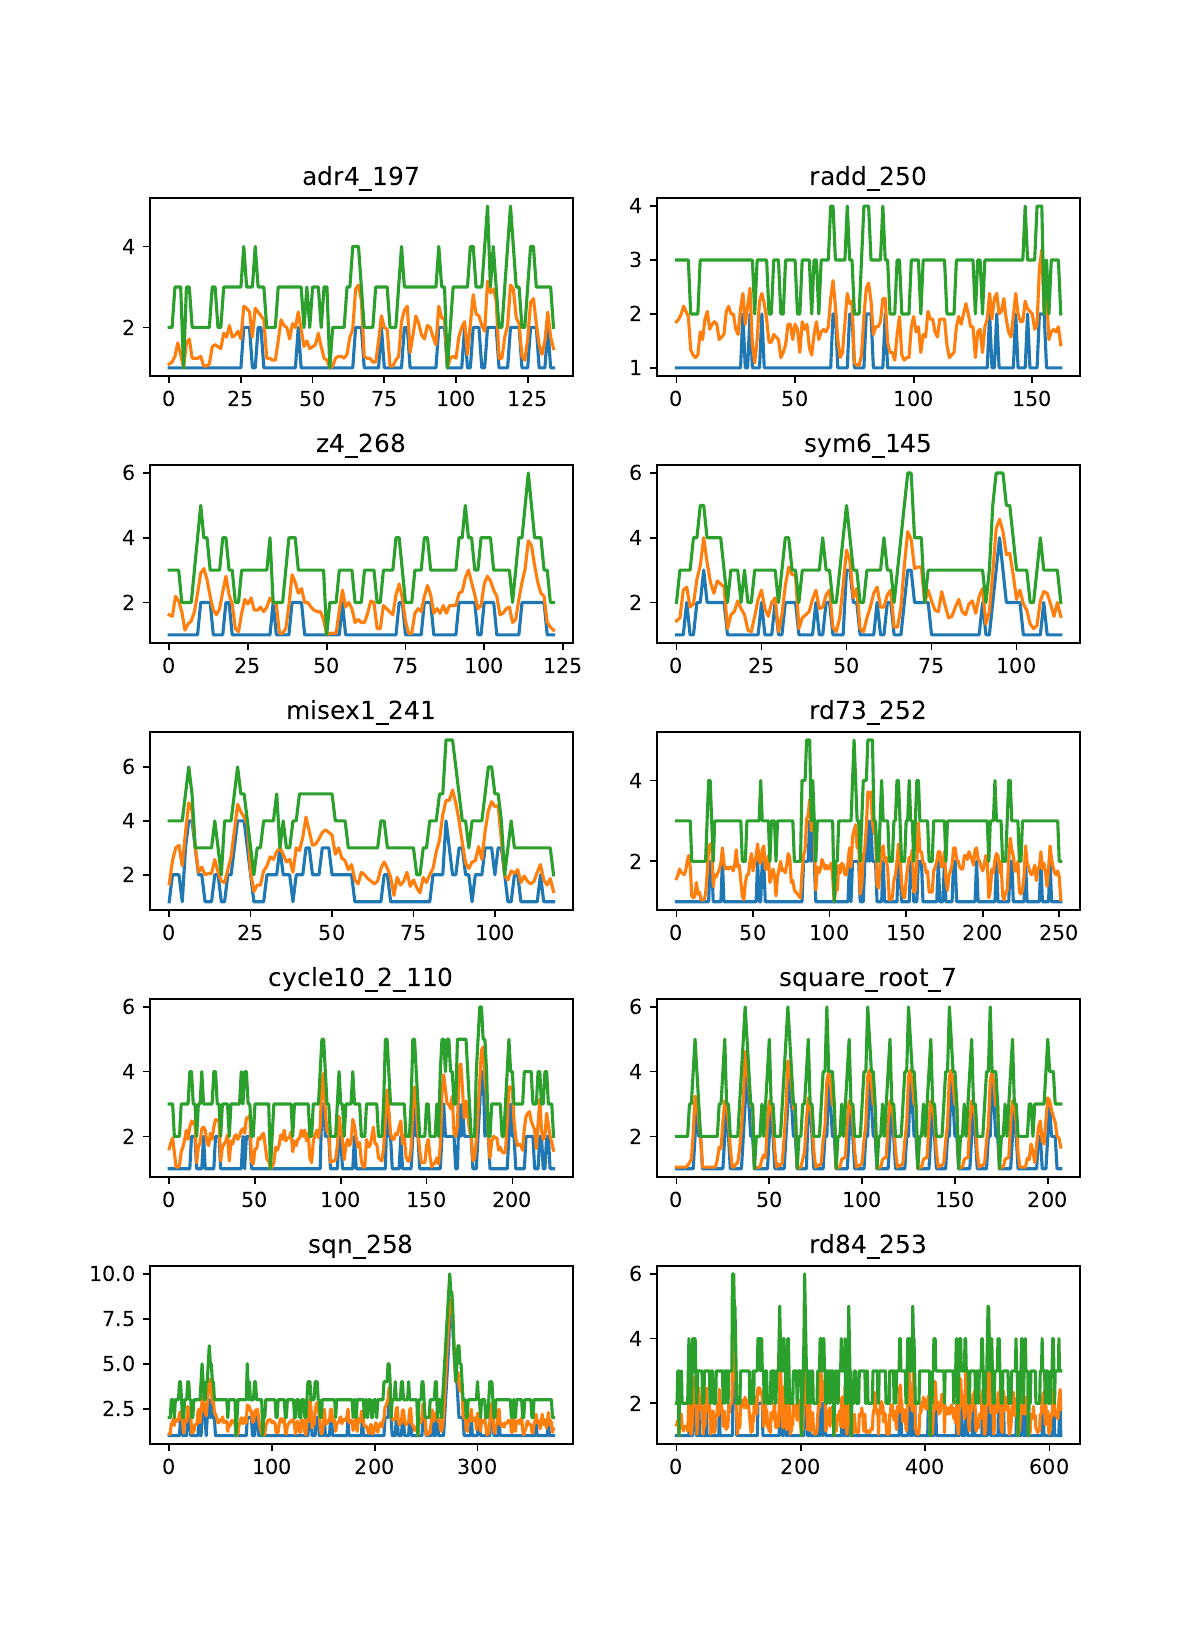}
	\caption{Results of search depths on small benchmark set with parameters setting as described in paper. The horizontal and vertical axis represent rounds for \emph{Decision} and search depth, respectively. The green, orange and blue line represent, respectively, the maximum, average and minimum depth among all \emph{Selection}s before each \emph{Decision} .}
	\label{fig:depth_play20}
\end{figure}

% \begin{figure}
% 	\centering
% 	\includegraphics[width=0.7\textwidth]{fig_depth_play_80_no_sim.pdf}
% 	\caption{Results of search depths on small benchmark set with \emph{Simulation} invalided and parameter $\chi_0$ setting to 80. The horizontal and vertical axis represent rounds for \emph{Decision} and search depth, respectively. The green, orange and blue line represent, respectively, the maximum, average and minimum depth among all \emph{Selection}s before each \emph{Decision} . The aggregated number of gates in output circuits is 70027.}
% 	\label{fig:depth_play80_no_sim}
% \end{figure}

%Comparison of MCTS-Depth with \tket \cite{CowtanRouting} on IBM Q20 with naive initial mappings.

\begin{longtable}[c]{cccccccc}
\caption{Comparison of MCTS-Depth with \tket \cite{CowtanRouting} on IBM Q20 with naive initial mappings.}
%\label{tab:my-table}\\
\\
\hline
\begin{tabular}[c]{@{}c@{}}Circuit\\      Name\end{tabular} & \begin{tabular}[c]{@{}c@{}}Input\\      Gates\end{tabular} & \begin{tabular}[c]{@{}c@{}}Input\\      Depth\end{tabular} & \begin{tabular}[c]{@{}c@{}}Gates   Added\\      Pytket\end{tabular} & \begin{tabular}[c]{@{}c@{}}Depth Added\\      Pytket\end{tabular} & \begin{tabular}[c]{@{}c@{}}Gates Added\\      MCTS-Depth\end{tabular} & \begin{tabular}[c]{@{}c@{}}Depth Added\\      MCTS-Depth\end{tabular} & Improvement \\
\hline
\endhead
%
graycode6\_47 & 5 & 5 & 9 & 3 & 9 & 3 & 0.0\% \\
xor5\_254 & 7 & 5 & 15 & 10 & 18 & 5 & 50.0\% \\
ex1\_226 & 7 & 5 & 15 & 10 & 18 & 5 & 50.0\% \\
4gt11\_84 & 18 & 11 & 12 & 10 & 27 & 8 & 20.0\% \\
ex-1\_166 & 19 & 12 & 9 & 10 & 12 & 6 & 40.0\% \\
ham3\_102 & 20 & 13 & 12 & 13 & 18 & 8 & 38.5\% \\
4mod5-v0\_20 & 20 & 12 & 15 & 13 & 9 & 3 & 76.9\% \\
4mod5-v1\_22 & 21 & 12 & 15 & 17 & 21 & 9 & 47.1\% \\
mod5d1\_63 & 22 & 13 & 24 & 24 & 21 & 6 & 75.0\% \\
4gt11\_83 & 23 & 16 & 18 & 19 & 15 & 4 & 78.9\% \\
4gt11\_82 & 27 & 20 & 30 & 31 & 33 & 6 & 80.6\% \\
rd32-v0\_66 & 34 & 20 & 24 & 26 & 15 & 6 & 76.9\% \\
mod5mils\_65 & 35 & 21 & 30 & 27 & 21 & 6 & 77.8\% \\
4mod5-v0\_19 & 35 & 21 & 30 & 29 & 24 & 5 & 82.8\% \\
rd32-v1\_68 & 36 & 21 & 24 & 27 & 18 & 5 & 81.5\% \\
alu-v0\_27 & 36 & 21 & 30 & 29 & 21 & 6 & 79.3\% \\
3\_17\_13 & 36 & 22 & 21 & 26 & 12 & 7 & 73.1\% \\
4mod5-v1\_24 & 36 & 21 & 36 & 34 & 18 & 7 & 79.4\% \\
alu-v1\_29 & 37 & 22 & 27 & 25 & 18 & 5 & 80.0\% \\
alu-v1\_28 & 37 & 22 & 30 & 33 & 24 & 6 & 81.8\% \\
alu-v3\_35 & 37 & 22 & 33 & 30 & 18 & 6 & 80.0\% \\
alu-v2\_33 & 37 & 22 & 27 & 28 & 21 & 6 & 78.6\% \\
alu-v4\_37 & 37 & 22 & 30 & 30 & 21 & 6 & 80.0\% \\
miller\_11 & 50 & 29 & 27 & 32 & 12 & 6 & 81.3\% \\
decod24-v0\_38 & 51 & 30 & 36 & 41 & 15 & 5 & 87.8\% \\
alu-v3\_34 & 52 & 30 & 45 & 48 & 24 & 7 & 85.4\% \\
decod24-v2\_43 & 52 & 30 & 36 & 42 & 15 & 4 & 90.5\% \\
mod5d2\_64 & 53 & 32 & 51 & 53 & 36 & 10 & 81.1\% \\
4gt13\_92 & 66 & 38 & 54 & 63 & 42 & 9 & 85.7\% \\
4gt13-v1\_93 & 68 & 39 & 45 & 50 & 48 & 11 & 78.0\% \\
one-two-three-v2\_100 & 69 & 40 & 54 & 62 & 30 & 10 & 83.9\% \\
4mod5-v1\_23 & 69 & 41 & 60 & 66 & 66 & 11 & 83.3\% \\
4mod5-v0\_18 & 69 & 40 & 51 & 61 & 48 & 13 & 78.7\% \\
one-two-three-v3\_101 & 70 & 40 & 57 & 61 & 30 & 13 & 78.7\% \\
4mod5-bdd\_287 & 70 & 41 & 45 & 51 & 27 & 6 & 88.2\% \\
decod24-bdd\_294 & 73 & 40 & 45 & 48 & 27 & 9 & 81.3\% \\
4gt5\_75 & 83 & 47 & 63 & 63 & 57 & 14 & 77.8\% \\
alu-v0\_26 & 84 & 49 & 72 & 76 & 42 & 7 & 90.8\% \\
rd32\_270 & 84 & 47 & 51 & 53 & 45 & 13 & 75.5\% \\
alu-bdd\_288 & 84 & 48 & 39 & 32 & 75 & 10 & 68.8\% \\
decod24-v1\_41 & 85 & 50 & 69 & 76 & 30 & 8 & 89.5\% \\
4gt5\_76 & 91 & 56 & 66 & 74 & 54 & 10 & 86.5\% \\
4gt13\_91 & 103 & 61 & 63 & 65 & 39 & 7 & 89.2\% \\
4gt13\_90 & 107 & 65 & 69 & 70 & 45 & 7 & 90.0\% \\
alu-v4\_36 & 115 & 66 & 72 & 84 & 54 & 17 & 79.8\% \\
4gt5\_77 & 131 & 74 & 54 & 48 & 45 & 14 & 70.8\% \\
one-two-three-v1\_99 & 132 & 76 & 102 & 107 & 72 & 17 & 84.1\% \\
rd53\_138 & 132 & 56 & 54 & 46 & 117 & 29 & 37.0\% \\
one-two-three-v0\_98 & 146 & 82 & 84 & 99 & 96 & 18 & 81.8\% \\
4gt10-v1\_81 & 148 & 84 & 102 & 109 & 90 & 13 & 88.1\% \\
decod24-v3\_45 & 150 & 84 & 123 & 136 & 90 & 15 & 89.0\% \\
aj-e11\_165 & 151 & 86 & 84 & 89 & 84 & 17 & 80.9\% \\
4mod7-v0\_94 & 162 & 92 & 99 & 112 & 93 & 17 & 84.8\% \\
alu-v2\_32 & 163 & 92 & 105 & 117 & 63 & 18 & 84.6\% \\
4mod7-v1\_96 & 164 & 94 & 102 & 117 & 72 & 17 & 85.5\% \\
cnt3-5\_179 & 175 & 61 & 162 & 91 & 159 & 28 & 69.2\% \\
mod10\_176 & 178 & 101 & 87 & 90 & 105 & 20 & 77.8\% \\
4gt4-v0\_80 & 179 & 101 & 96 & 102 & 69 & 10 & 90.2\% \\
4gt12-v0\_88 & 194 & 108 & 114 & 111 & 54 & 14 & 87.4\% \\
0410184\_169 & 211 & 104 & 147 & 112 & 132 & 20 & 82.1\% \\
4\_49\_16 & 217 & 125 & 132 & 150 & 102 & 13 & 91.3\% \\
4gt12-v1\_89 & 228 & 130 & 126 & 116 & 63 & 14 & 87.9\% \\
4gt4-v0\_79 & 231 & 132 & 75 & 63 & 69 & 9 & 85.7\% \\
hwb4\_49 & 233 & 134 & 159 & 174 & 93 & 19 & 89.1\% \\
4gt4-v0\_78 & 235 & 137 & 81 & 68 & 105 & 15 & 77.9\% \\
mod10\_171 & 244 & 139 & 162 & 171 & 90 & 16 & 90.6\% \\
4gt12-v0\_87 & 247 & 131 & 90 & 80 & 84 & 23 & 71.3\% \\
4gt12-v0\_86 & 251 & 135 & 93 & 82 & 72 & 20 & 75.6\% \\
4gt4-v0\_72 & 258 & 137 & 165 & 160 & 66 & 15 & 90.6\% \\
4gt4-v1\_74 & 273 & 154 & 198 & 217 & 111 & 24 & 88.9\% \\
mini-alu\_167 & 288 & 162 & 210 & 235 & 132 & 31 & 86.8\% \\
one-two-three-v0\_97 & 290 & 163 & 225 & 259 & 111 & 39 & 84.9\% \\
rd53\_135 & 296 & 159 & 165 & 165 & 138 & 29 & 82.4\% \\
ham7\_104 & 320 & 185 & 63 & 46 & 102 & 26 & 43.5\% \\
decod24-enable\_126 & 338 & 190 & 177 & 192 & 105 & 27 & 85.9\% \\
mod8-10\_178 & 342 & 193 & 156 & 162 & 57 & 15 & 90.7\% \\
4gt4-v0\_73 & 395 & 227 & 282 & 312 & 87 & 22 & 92.9\% \\
ex3\_229 & 403 & 226 & 234 & 234 & 69 & 20 & 91.5\% \\
mod8-10\_177 & 440 & 251 & 195 & 188 & 105 & 19 & 89.9\% \\
alu-v2\_31 & 451 & 255 & 303 & 331 & 141 & 37 & 88.8\% \\
C17\_204 & 467 & 253 & 210 & 214 & 99 & 24 & 88.8\% \\
rd53\_131 & 469 & 261 & 240 & 258 & 75 & 28 & 89.1\% \\
alu-v2\_30 & 504 & 285 & 273 & 289 & 99 & 43 & 85.1\% \\
mod5adder\_127 & 555 & 302 & 255 & 263 & 138 & 36 & 86.3\% \\
rd53\_133 & 580 & 327 & 348 & 365 & 123 & 34 & 90.7\% \\
majority\_239 & 612 & 344 & 219 & 229 & 150 & 31 & 86.5\% \\
ex2\_227 & 631 & 355 & 345 & 361 & 156 & 28 & 92.2\% \\
cm82a\_208 & 650 & 337 & 330 & 303 & 195 & 59 & 80.5\% \\
sf\_276 & 778 & 435 & 348 & 365 & 111 & 36 & 90.1\% \\
sf\_274 & 781 & 436 & 339 & 417 & 51 & 26 & 93.8\% \\
con1\_216 & 954 & 508 & 501 & 512 & 291 & 66 & 87.1\% \\
rd53\_130 & 1043 & 569 & 456 & 442 & 261 & 65 & 85.3\% \\
f2\_232 & 1206 & 668 & 558 & 572 & 285 & 56 & 90.2\% \\
rd53\_251 & 1291 & 712 & 627 & 693 & 303 & 65 & 90.6\% \\
hwb5\_53 & 1336 & 758 & 510 & 537 & 384 & 97 & 81.9\% \\
radd\_250 & 3213 & 1781 & 1341 & 1345 & 882 & 160 & 88.1\% \\
rd73\_252 & 5321 & 2867 & 1983 & 1952 & 1347 & 318 & 83.7\% \\
cycle10\_2\_110 & 6050 & 3386 & 2697 & 2788 & 1518 & 344 & 87.7\% \\
hwb6\_56 & 6723 & 3736 & 2598 & 2688 & 1563 & 390 & 85.5\% \\
cm85a\_209 & 11414 & 6374 & 4083 & 4032 & 2529 & 588 & 85.4\% \\
rd84\_253 & 13658 & 7261 & 5853 & 5776 & 3954 & 963 & 83.3\% \\
root\_255 & 17159 & 8835 & 7137 & 7209 & 3957 & 1135 & 84.3\% \\
mlp4\_245 & 18852 & 10328 & 8607 & 8295 & 5535 & 1210 & 85.4\% \\
urf2\_277 & 20112 & 11390 & 10524 & 10247 & 10224 & 2674 & 73.9\% \\
sym9\_148 & 21504 & 12087 & 8190 & 8495 & 1290 & 133 & 98.4\% \\
hwb7\_59 & 24379 & 13437 & 11523 & 11718 & 5178 & 1227 & 89.5\% \\
clip\_206 & 33827 & 17879 & 13992 & 13897 & 8670 & 2306 & 83.4\% \\
sym9\_193 & 34881 & 19235 & 15213 & 15159 & 7473 & 1742 & 88.5\% \\
dist\_223 & 38046 & 19694 & 15576 & 15656 & 8622 & 2581 & 83.5\% \\
sao2\_257 & 38577 & 19563 & 14928 & 14852 & 8691 & 2739 & 81.6\% \\
urf5\_280 & 49829 & 27822 & 22113 & 21636 & 19401 & 5154 & 76.2\% \\
urf1\_278 & 54766 & 30955 & 24948 & 24119 & 20541 & 5564 & 76.9\% \\
sym10\_262 & 64283 & 35572 & 28071 & 27923 & 15855 & 3369 & 87.9\% \\
hwb8\_113 & 69380 & 38717 & 26043 & 26039 & 17043 & 3462 & 86.7\% \\
Summary & 554497 & 303469 & 237471 & 236312 & 151530 & 37794 & 84.0\% \\
\hline
\end{longtable}
